# Supplementary material for: Cut Costs, Not Accuracy: LLM-Powered Data Processing with Guarantees
Source: arXiv:2509.02896 source file (2025-09-12)
Supplement: Supplementary file 1 [file proof_precision.tex]

\section{Proofs for Precision Target Querie}
\subsection{Uniform Sampling}
An approach similar to recall is to adjust the target precision provided to us to a new threshold $\tau$, so that if for a proxy score $P_S(\rho)\geq \tau$ then $P_D(\rho)\geq T$ with high probability. We first discuss this approach, and then show that instead of adjusting the threshold, using the iterative method, similar to Sec.X, we can provide results with much better utility. 

\subsubsection{Naive  with Union bound}
The algorithm is similar to recall. Let 
$$\rho_S^\tau=\min\{\rho, P_S(\rho)\geq \tau\},$$
where $\tau>T$ is the adjusted target. Then, similar to before, we return the set of points whose proxy score is at last $\rho_S^\tau$.

An important difference between the above procedure, comparing precision and recall, is that precision is not monotonically decreasing. This is important for the following reason. Consider $r$ different thresholds in sorted order, $\bar{\rho}_1, ..., \bar{\rho}_r$ where, for all $i\in[r]$ $P_D(\bar{\rho}_i)<T$. We can have $P_S(\rho_i)>T$ while $P_S(\bar{\rho}_j)<T$ for $i\neq j$. This contrasts with recall, where  if $R_S(\rho_i)<T$ then $R_S(\rho_j)<T$ for $\rho_i>\rho_j$. This effectively allows us to study a single event $R_S(\bar{\rho}_D)>T$ to study correctness of our algorithm. For precision, on the other hand, we need to consider all of $P_S(\bar{\rho}_j)>T$. To do so, we can simply use the union bound to study  $P_S(\bar{\rho}_j)>\tau$ for each $i$ separately, and use the union bound to bound the union of the events. Since union bound simply bounds the probability of failure by sum of failure probabilities, the more events we consider, the more confident about each event we need to be to achieve the given total failure probability of $\delta$. As such, we introduce the parameter $M$ that decides how many events to consider. Let $\mathcal{E_M}=\{\frac{i}{M}, i\in[M]\}$, so that
\begin{align*}
    \hat{\rho}_S^\tau=\min\{\rho\in\mathcal{E_M}, P_S(\rho)\geq \tau\}.
\end{align*}
Maybe also mention non-union bound, but that we didn't see much benefit and its complex so we avoid presenting it
We have 
\begin{lemma}
Using adjusted target $\tau=T+\sqrt{\frac{\log(M/\delta)}{2k}}$, the adjusted threshold algorithm returns a set that matches target $T$ with probability at lest $\delta$
\end{lemma}

\textit{Proof}. For any $i$, the algorithm checks if $P_S(\frac{i}{M})\geq \tau$. The algorithm returns precision less than $T$ if for some $i$, $P_S(\frac{i}{M})\geq \tau$ but $P_D(\frac{i}{M})< T$. Note that $P_D(\frac{i}{M})=\mathds{E}(P_S(\frac{i}{M}))$, so we have
\begin{align}
\mathds{P}(P_S(\frac{i}{M})-P_D(\frac{i}{M})\geq\epsilon)\leq \exp{(-\frac{k\epsilon^2}{2})}
    \end{align}

We are only concerned with cases where $P_D(\frac{i}{M})< T$. Substituting this, we have 
\begin{align}
\mathds{P}(P_S(\frac{i}{M})\geq T+\epsilon)\leq \exp{(-\frac{k\epsilon^2}{2})}.    
\end{align}


Setting the right hand side to be $\frac{\delta}{M}$ and substituting $\tau$ we have
$$
\mathds{P}(P_S(\frac{i}{M})\geq \tau)\leq \frac{\delta}{M}
$$
for any $i$ where $P_D(\frac{i}{M})< T$. In the worst case, $P_D(\frac{i}{M})< T$ is true for all $i$, and using the union bound across all $i$, the probability that for any $i$ we have $P_S(\frac{i}{M})\geq \tau$ is bounded by $\delta$, proving the result.\qed

\textbf{Discussion}. 
The adjusted threshold is often much larger than the original threshold due to the factor $M$.  To try to avoid this, we take a deeper look into the analysis. Consider the $M$ events $P_S(\frac{i}{M})\geq \tau$ studies. In the wort-csae $P_D(\frac{i}{M})< T$ can hold for all $i$, which means we need to study the union of the $M$ events. Moreover, we can have $P_D(\frac{i}{M})>T-\epsilon$ for any small $\epsilon$ can hold for all $i$. These two characteristic of the analysis, although possible in the worst-case, are not realistic. Precision, much like recall, does in fact often follow a generally reducing pattern. Moreover, often, the range of values the hover around $T$ is small, so we don't need to consider settings where precision is small at the begining and then suddenly gets better towards the end. 

\subsubsection{Iterative without union bound}
To resolve the avoid issues, we observe that an iterative algorithm can significantly improve accuracy in practice, without having to resort to using a union bound. 

The iterative algorithm performs similarly to Alg.~\ref{alg:iterative_recall}, but now $\lambda(S, S[i])=\mathcal{L}(\{\mathds{I}[\mathcal{O}(x)=1], x\in S, x\geq\rho\})-T$. This looks very similar to the threshold-based algorithm, with one main difference. The algorithm stops at the first threshold where it estimates the mean can go below $T$, while threshold based methods attempt to find the smallest $\rho$ at which precision is above $T$. Intuitively, iterative algorithm attempts to the largest $T$ after which precision drops below $T$, while threshold based method attempts to find the smallest $\rho$ after which the precision drops below $T$. Below, we show that this simple change in the algorithm can help significantly improve accuracy. 

\begin{lemma}
    Using $\lambda=\mathcal{L}(\{\mathds{I}[\mathcal{O}(x)=1], x\in S, x\geq\rho\})-T$, we have that the algorithm returns a set that matches the precision target with probability at least $1-\delta$.
\end{lemma}

\textit{Proof}. Define 
\begin{align}\label{eq:rho_bar_precision}
    \bar{\rho}_D=\max(\{\rho;\rho\in[0, 1], P_D(\rho)<T,P_D(\rho')\geq T,\,\forall\rho'>\rho\}).
\end{align}
$\bar{\rho}_D$ is the first proxy score at which the model precision drops below $T$ when iterating through proxy scores in descending order. We consider the event where $\lambda(S, \bar{\rho}_D)\geq 0$.  Note that if the algorithm fails, it must be that $\lambda(S, \bar{\rho}_D)\geq 0$. Although $\lambda(S, \bar{\rho}_D)\geq 0$ does not necessarily imply failure, we can bound the probability of failure by $\mathds{P}(\lambda(S, \bar{\rho}_D)\geq 0).$ Using Lemma~\ref{lemma:lb} and the fact that $R_D(\bar{\rho}_D)<T$, we have
$$\mathds{P}(\mathcal{L}(\{\mathds{I}[\mathcal{O}(x)=1], x\in S, x\geq\bar{\rho}_D\})>T)\leq \delta$$
which proves the results.\qed




CAN PROBABLY JUST PLOT THE VALUES, CAN PERHAPS FORMALLY STATE AT LEAST THE PROPERTY WE're INTERESTED IN


\subsection{Iterative sampling}
Finally, taking into account the properties of precision, we can improve the sampling procedure. The main observation here is that if the algorihtm stops at a threshold $\rho$, it will not have looked at any labeled point with proxy score smaller than $\rho$, effectivly wasting labeling budget. To avoid that, we modify the sampling procedure as follows. 

Let $s$ be a sampling step size and $m$ be an evaluation step size, and let $\mathcal{E}_s\{\frac{i}{s}, \forall i\in [s]\}$ and $\mathcal{E}_M\{\frac{i}{M}, \forall i\in [M]\}$. Intuitively, the algorithm expands the domain it samples over according to $\mathcal{E}_s$, and searches over potential proxy thresholds in $\mathcal{E}_M$ to see if such thresholds are expected to meet the target precision. 




\begin{lemma}
    Alg~\ref{alg:iterative_sample_precision} meets precision target with probability at least $1-\delta$.
\end{lemma}

\textit{Proof}. Consider $\bar{\rho}_D$ as defined in Eq.~\ref{eq:rho_bar_precision}, and let $\bar{i}=\max \{i; \frac{i}{M}\leq \bar{\rho}_D\}$. The algorithm fail only if $\lambda(S, \frac{\bar{i}}{m})\geq 0$ by the end of
