# Supplementary material for: Cut Costs, Not Accuracy: LLM-Powered Data Processing with Guarantees
Source: arXiv:2509.02896 source file (2025-09-12)
Supplement: Supplementary file 2 [file proof_recall.tex]

\section{Detailed Recall Target Queries Proof}
\subsection{Why Not Importance Sampling}

%\subsection{\name{}$_R$-I: \name{} with Importance Sampling}
How Theorem~\ref{thm:adj_target_exact} adjusts the target depends on $k^+$, the number of observed positive samples. The smaller $k^+$ is, the larger the adjusted target will be and the worse the final precision will be. Thus, to obtain better results, ideally, our sampling procedure needs to sample as many positives as possible. %This means quality of the result set returned by Theorem~\ref{thm:adj_target_exact} depends on how many positives there are in the dataset. When the total number of positives is small compared with data size, Theorem~\ref{thm:adj_target_exact} may need too many samples to reach a meaningful accuracy. In such a setting, we may want to change our sampling strategy to ensure more positives .

\textbf{Importance Sampling.} One way to achieve this is by using the proxy scores for sampling. If the proxy model is well-calibrated, then by sampling records with higher proxy scores, we can hope to sample more positives. This can be achieved by importance sampling, where the probability of sampling a records become proportional to proxy score for that record. Specifically, let%\sep{write down sampling procedure}% if the sampling strategy weighs elements based on the proxy scores.
$$
\mathcal{W}(x)=\frac{\mathcal{S}(x)}{\sum_{x\in D}\mathcal{S}(x)},
$$
the normalized proxy scores, so that $\mathcal{W}$ specifies a valid p.m.f over the elements of $D$. During importance sampling, each record $x\in D$ has probability $\mathcal{W}(x)$ to be sampled. 
%We discuss two solutions to do so. Our first solution uses naive importance sampling, similar to XX, but unlike XXX provides theoretical guarantees. As we discuss below, naive importance sampling can significantly increase variance if there is even small calibration error in the model. This means, an algorithm that provides theoretical guarantees while using naive importance sampling has almost no utility. To address this issue, we propose clamped importance sampling, tha combined clamping with importance sampling to reduce the variance. This approach increases bias but reduces variance, where we quantify the bias in terms of model calibration error. This approach provides theoretical guarantees that depend on the model calibration error.

\textbf{Discriminator-Based Selection Algorithm}. Importance sampling creates new challenges. Because the samples are non-uniform, we must adjust our observations to account for this non-uniformness and cannot simply use $\mathfrak{R}_S(\rho)$ as the sample recall estimate. For reasons we discuss in more depth in Sec XX, finding a suitable adjustment is non-trivial, and simple adaptations of our previous threshold adjustment algorithm and analysis cannot be applied to this sampling procedure. 

Instead of using an adjusted target to choose the cascade threshold, we use a discriminator function, $\lambda(S, \rho)$. This discrimination function is a generalization of target adjustment and fulfills a similar role. Specifically, $\lambda(S, \rho)$ decides, based on the observed sample $S$, whether for the threshold $\rho$ the true recall $\mathfrak{R}_D(\rho)$ meets the target $T$ or not. Note that setting $\lambda(S, \rho)=\mathfrak{R}_S(\rho)-(\tau-T)$, we obtain Alg.~\ref{alg:thresh_recall}, so that Alg.~\ref{alg:iterative_recall} is a generalization to allow solutions beyond threshold adjustment. 

\textbf{\name{$_R$-I}}. The discriminator-based approach allows us to use Lemma~\ref{lemma:lb}. Specifically, given the sample set, $S$, let $$S^\rho=\{\mathds{I}[x\geq \rho], x\in S^+\}$$ and set $\lambda(S, \rho)=\mathds{L}(S^\rho, \delta)$. $\mathds{L}$ provides a probabilistic lower bound on the true mean of $S^\rho$, so that Alg.~\ref{alg:iterative_recall} would choose a $\rho$ such that expected value of elements of $S^\rho$ is more than $T$. Indeed, this algorithm would've been valid if $\mathds{E}_{S\sim W}[\frac{\sum_{x\in S^\rho}x}{|S^\rho|}]=\mathds{R}_D(\rho)$. However, because of importance sampling, this statement is not true, and we need to adjust $S^\rho$ to account for the non-uniform sampling. The following theorem shows how this can be done, specifically presenting a $\lambda$ function for which Alg.~\ref{alg:iterative_recall} is valid. 

%setting  from Lemma~\ref{lemma:lb}
%To address these challenges, \sep{better connet}, to relate observed mean to true mean, we use Lemma~\ref{lemma:lb}. An important consequence of using Lemma~\ref{lemma:lb} is that we can no longer provide a data-independent adjusted threshold $\tau$, since Lemma~\ref{lemma:lb} relates to the data distribution for each specific $\rho$. 
%The following Theorem shows that for an appropriate choice of $\lambda$, set based on Lemma~\ref{lemma:lb}, we can use Alg.~\ref{alg:iterative_recall} to return results with the desired theoretical guarantee.
%Moreover, to account for importance sampling, we adjust our observation using some transformation $f$, as specified in the following Theorem. 

%Thus, in our analysis for importance sampling, we use Lemma~\ref{lemma:lb} to relate mean of observation to their true mean. 

%This leads to two important changes to our methodology, first, the analysis in Theorem~\ref{thm:adj_target_exact} that allowed us to obtain tight bounds is no longer possible. Although we can still use Hoeffding inequality as a substitute, similar to Lemma~\ref{lemma:adj_target_hoef}, such a result will lead to loose bounds, compromising accuracy. On the other hand, bound such as the Central Limit Theorem considers data variance but only holds in the limit. This means we cannot simply chose a data independent adjusted target and follow Alg.~\ref{alg:thresh_recall}. 

%e note that Theorem 3 by \cite{waudby2024estimating} is more general, and among other generalizations provides a two-sided confidence interval (not just a lower bound on mean as Lemma~\ref{lemma:lb} states). In our analysis, we are only interested in lower bounds and thus have stated a simplification of the result.  

%Note that, since, Lemma~\ref{lemma:lb} provides a data-pendent function


%To do so, we devise an iterative threshold selection algorithm, presented in Alg.~\ref{alg:iterative_recall}, which is a generalization of Alg.~\ref{alg:thresh_recall}. It iterates over the data points in ascending order and uses a \textit{discriminator function}, $\lambda(S, \rho)$, to decide when to stop. This discriminator function decides, given a set $S$ and threshold 
%When setting $\lambda(S, \rho)=R_S(\rho)-\tau$ (for either choice of $\tau$ from Lemma~\ref{lemma:adj_target_hoef} or Theorem~\ref{thm:adj_target_exact}), Alg.~\ref{alg:thresh_recall} becomes equivalent to Alg.~\ref{alg:iterative_recall} (since $\mathfrak{R}_S(\rho)-\tau$ is monotonically decreasing). However, Alg.~\ref{alg:iterative_recall} allows non-threshold-based decision making. Intuitively, $\lambda(S, \rho)$ is a function that helps us decide if $\rho$ is a valid cascade threshold. A suitable $\lambda$ ensures that $\lambda(S, \rho)\geq 0$ for any $\rho$ s.t. $\mathfrak{R}_D(\rho)\geq T$, and $\lambda(S, \rho)< 0$ for any $\rho$ where $\mathfrak{R}_D(\rho)< T$. Since $\mathfrak{R}_D(\rho)$ is not known, $\lambda$ should be chosen 

%Here, we're interested in setting $\lambda(S, \rho)$ to be be function that finds a lower bound $L$ for $\mathds{E}[R_S(\rho)]-T$ with high probability. The algorithm would then find a value of $\rho$ for which $L\geq 0$, which implies  $\mathds{E}[R_S(\rho)]\geq T$.



\begin{theorem}\label{theorm:importance_sampling}
    Let $\lambda(S, \rho)=\mathds{L}({Z}^\rho, \delta)$ where $${Z}^\rho=\{\psi\frac{\mathds{I}[x>\rho]-T}{\mathcal{S}(x)}+T, x\in S^+\},\; \psi=\min_{x\in D^+}\mathcal{S}(x)
    $$
    %$$
    %\text{with}\; \psi\; \text{as either}\; \psi=\min_{x\in D}\mathcal{P}(x)\; \text{or}\; \psi=\min_{x\in D^+}\mathcal{P}(x).
    %$$
    
    Then, Alg.~\ref{alg:iterative_recall} returns a set of elements with recall less than $T$ with probability at most $\delta$.
\end{theorem}

Comparing $Z^\rho$ with $S^\rho$ we observe the adjustment needed due to importance sampling. We discuss in more depth, in Sec XXX, why a typical adjustment commonly done in importance sampling does not provide guarantees in our case. 
%Theorem~\ref{theorm:importance_sampling} uses $\mathds{L}$ from Lemma~\ref{lemma:lb}.
Also note that when $\psi=\min_{x\in D^+}\mathcal{S}(x)$ is not known, it can be replaced with $\psi=\min_{x\in D}\mathcal{S}(x)$, as we do in practice. 

\sep{can we just do something similar to iterative sampling? Or do assumption + iterative sampling?}



\textbf{Challenges with Importance Sampling.} Observe that in Lemma~\ref{theorm:importance_sampling} our random variables depend on $\frac{1}{\mathcal{S}(x)}$. This means if the proxy score for a positive sample is lower, the value of the random variable can significantly explode, leading to high variance in the estimator. More formally, 
\begin{lemma}\label{lemma:importance_variance} Consider a random variable $Z\in Z^\rho$ from Lemma~\ref{theorm:importance_sampling} for any $\rho\in[0, 1]$. We have\sep{double check $\rho=0, 1$}
\begin{align*}
    \frac{\varkappa_1}{\varkappa_2}+\frac{T^2}{\varkappa_2}\sum_{x<\rho}\frac{1}{\mathcal{S}(x)}\leq \mathtt{Var}(Z)\leq \frac{\varkappa_1}{\rho\varkappa_2}+\frac{T^2}{\varkappa_2}\sum_{x<\rho}\frac{1}{\mathcal{S}(x)},
\end{align*}
for $\varkappa_1=|D^+|((1-T)^2R_D(\rho)+T-R_D(\rho))$ and $\varkappa_2=\sum_{x\in D}\mathcal{S}(x)$.
\end{lemma}
Importantly, observe the dependence on $\frac{1}{\mathcal{P}(x)}$ in Lemma~\ref{lemma:importance_variance} for $x<\rho$. Note the higher the variance, the more difficult it is to estimate the sample mean, so that $\mathds{L}(Z^\rho, \delta)$ can provide vacuous bounds for high variance random variables. 
%Recall that our analysis in Lemma~\ref{theorm:importance_sampling} depended on $Z_i^{\bar{\rho}_D}$. Using $\bar{\rho}_D$ in Lemma~\ref{lemma:importance_variance}, implies that the approach is particularly sensitive to proxy scores smaller than $\bar{\rho}_D$ for positive records. By definition of $\bar{\rho}_D$, more than $1-T$ percent of the positives are have scores smaller than $\bar{\rho}_D$. 
This means even if one positive record has $\mathcal{S}(x)$ close to zero, $Var(Z)$ becomes extremely large, leading to an estimator with little utility. Since, in practice, even if models are in general calibrated, they can be uncalibrated for a few samples, $\mathcal{S}(x)$ can be small for positive samples. Thus, using the importance sampling approach discussed above performs poorly.




\subsection{Uniform sampling and adjusted target}
We are given a recall target, $T$, and our goal is to find a proxy threshold, $\rho_S$, using a sample, $S$, of the data such that $\mathds{P}_{S~D}(R_D(\rho_S)<T)<\delta$.

Define $R_S(\rho)=\frac{\{x\in S, x\geq \rho, O(x)=1\}}{\{x\in S, O(x)=1\}}$. That is, $R_S(\rho)$ is the recall of filtering data points based on $\rho$ with respect to the set $S$. 

A straightforward approach without a theoretical guarantee is to set 
$$\rho_S=\max\{\rho, R_S(\rho)\geq T\}.$$ 
That is, to find the largest proxy threshold on the observed samples such that observed recall is at least $T$. Such an approach does not provide any guarantees, since the observed samples deviate from the ground-truth, and we may observe, at a specific threshold, recall that is larger than the ground-truth. 


To resolve the above issue, we can set 
$$\rho_S^{\tau}=\max\{\rho, R_S(\rho)\geq \tau\},$$
where $\tau>T$ is an \textit{adjusted} target. Here, rather than using the user provided target $T$, we find the largest proxy threshold such that the observed recall is at least equal the adjusted target $\tau$. Using an adjusted target $\tau$ larger than $T$ is done to adjust for sampling error. Intuitively, $\tau$ needs to be set so that if the observed recall is at least $\tau$, the true recall is at least $T$ with high probability. %For this approach to be statistically valid, we need to show that if the observed recall is at least $\tau$, then the true recall is at least $T$ with high probability. 

Bring up alg XXX.

The main result in this section is to show how to set the adjusted target $\tau$ to ensure Alg.~\ref{alg:thresh_recall} meets the recall target $T$ with probability at least $\delta$.

\begin{theorem}\label{thm:adj_target}
Alg.~\ref{alg:thresh_recall} meets the target threshold with the desired probability when choosing adjusted target, $\tau$ as $\tau_C$ or $\tau E$, where
\begin{align*}
    \tau^C=T+\sqrt{\frac{\log(1/\delta)}{2k^+}},\quad \quad \tau^E=\frac{1}{k^+}\min\{x, q(x)\leq \delta\}
\end{align*}
and $q(x)=\mathds{P}(\mathcal{B}(k^+, T)\geq x)$ is the tail probability of a binomial distribution with parameters $k^+$ and $T$. That is, $\mathds{P}_{S\sim D}(R_D(\rho^t_S)< T)\leq \delta$ for either choices of $\tau=\tau^C$ or $\tau=\tau^E$.
\end{theorem}

Theorem~\ref{thm:adj_target} presents two methods to set the adjusted target. $\tau^C$ provides a closed-form solution using concentration bounds while $\tau^E$, shows how to adjust the target using exact computations. The rest of this section discusses the proof of Theorem~\ref{thm:adj_target}

XXX Maybe add a figure showing the difference between the two and Kang et al XXXXX
XXX Maybe add a tightness result XXXX

\subsubsection{Guarantees Through Target Adjustment}

To make the above discussion precise, define 
\begin{align}%\label{eq:rho_d}
\bar{\rho}_D=\min\{\rho, R_D(\rho)< T\}.    
\end{align}
We don't know the value of $\bar{\rho}_D$, but we use it to quantify the probability of failure in our analysis. Specifically, given that the recall function, $R_D(\rho)$, is monotonically decreasing in $\rho$, we have $R_D(\rho)< T$ for $\rho\in[\bar{\rho}_D, 1]$ and  $R_D(\rho)\geq T$ for $\rho\in[0, \bar{\rho}_D)$ due to the definition of $\bar{\rho}_D$. Thus, we want to set $\tau$ so that $\rho_S^\tau\geq \bar{\rho}_D$ with high probability. We call such a value of $\tau$ a \textit{valid adjusted target}. More formally,

\begin{definition}
    An adjusted recall target $\tau\in[0, T)$ is \textit{valid} if 
    \begin{align}\label{eq:def_valid}
        \mathds{P}_{S\sim D}(R_S(\rho_D)\geq \tau)\leq \delta.
    \end{align}
\end{definition}

Note that if $R_S(\rho_D)\geq \tau$ holds for an observed sample $S$, then $\rho_S^\tau\geq \bar{\rho}_D$, and therefore $R_D(\rho_s^\tau)<T$, causing a failure in the algorithm. Thus, the validity of $\tau$ directly corresponds to the success of the algorithm. The following theorem states this formally.

\begin{lemma}
    Suppose $\tau$ is a valid adjusted target. Then, the adjusted target algorithm, Alg. XX fails with probability less than $\delta$. That is, $\mathds{P}_{S\sim D}(R_D(\rho^t_S)< T)\leq \delta.$
\end{lemma}

\textit{Proof}. Observe that Alg X fails only if $\rho_S^1\geq \bar{\rho}_D$. This is because $\rho_S^1< \bar{\rho}_D$ implies $R_D(\rho_S^1)\geq T$ by definition of $\bar{\rho}_D$. Thus, it remains to show $\mathds{P}(\rho_S^1\geq \bar{\rho}_D)\leq \delta$. Since the recall function $R_S(\rho)$ is monotonically decreasing in $\rho$, $R_S(\bar{\rho}_D)<\tau$ implies $R_S(\rho)<\tau\; \forall\rho\in[\bar{\rho}_D, 1]$. Consequently, $\rho_S^1\geq{\bar{\rho}_D}$ only if $R_S(\bar{\rho}_D)\geq \tau$. The probability of this event is bounded by $\delta$, which bounds probability of failure of Alg X by $\delta$ as well. \qed  %, $R_D(\rho_S^1)\leq R_D(\bar{\rho}_D)$ only if $\rho_S^1\leq \bar{\rho}_D$. That is, Alg X fails only i 


\subsubsection{Finding Valid Adjustments} Thus, it remains to find a valid value of $\tau$ that satisfies Eq.~\ref{eq:def_valid}. There are two challenges in such an analysis: (1) we don't know the value of $\bar{\rho}_D$, and (2) for a set of random observations $S$, both the numerator and the denominator of $R_S(\rho)$ are random variables. Our analysis below addresses the two challenges by utilizing the characteristics of the recall function. Regarding challenge (1) we show that, in fact, the exact value of $\bar{\rho}_D$ is not required for analysis and we can rely on the definition to still provide the desired guarantees. Regarding challenge (2) we show that a slight reformulation of the definition of recall can help avoid the need for analyzing the ratio of the random variables. We first discuss this reformulation, before presenting our results on how to find valid adjustments.

Specifically, note that recall on a set $S$ only depends on the positive samples. Consider the set $S^+\subseteq S$ where $S^+=\{x\in S, O(x)=1\}$, and let $k^+=|S^+|$. Then, $R_S(\rho)=\frac{\sum_{x\in S^+}\mathds{I}[x\geq \rho]}{k^+}$ only depends on the observations in $S^+$. Furthermore, given that $S^+$ is the subset of $S$ where we reject the samples with a negative label, elements of $S^+$ are sampled i.i.d and uniformly from the distribution of the elements with a positive label. As such, we have $$\mathds{E}_{X\sim D^+}[\mathds{I}[X\geq\rho]]=R_D(\rho),$$
Where $\mathds{I}$ is the indicator function.

Thus, only focusing on the positive observations allows us to estimate true recall using sum of i.i.d random and \{0, 1\} random variables. This naturally leads to attempting to analyze $R_S$ using concentration bounds. We first discuss such an approach using a concentration bound. Then, we show that, in fact, one can calculate answers using exact calculations, leading to much tighter bounds and, as a result, improved accuracy. 





%Our goal is to find the largest $\rho$ such that $R_D(\rho)\geq T$. We set $\rho$ based on the observed sample, i.e., $\rho=f(S)$ for some $f$. We would like to make sure $\mathds{P}_{S\sim D}(R_D(f(S))\leq T)\leq \delta$. Note . This makes the problem challenging since our goal is to estimate the ratio of two random variables, which is difficult. In fact, XXX analyses uses this ratio of the random variable in their analysis which leads to a looser analysis since the numerator and denominator are analyzed separately and the final result is combined using union bound. 

%Instead, looking into the characteristic of the recall, we show that it can be analyzed without having to resort to the ratio of the random variable.


\textbf{Valid Adjustments using Concentration Bounds.} Using the above reformulation, observe that $\mathds{E}_{S\sim D}R_S(\rho_D)=R_D(\rho_D)<T$. Thus, to analyze Eq.~\ref{eq:def_valid}, we can use a concentration bound to related the observed recall and expected recall at $R_D$. This is done in the following Lemma.


%Thus, a valid value of $\tau$ is a value for which the previous statement holds. Indeed, such a statement can be shown using standard concentration bounds, which provide a means to set $\tau$.

\begin{lemma}
    $\tau^C=T+\sqrt{\frac{\log(1/\delta)}{2k^+}}$ is a valid adjusted target, i.e., $$\mathds{P}_{S\sim D}(R_S(\rho_D)\geq \tau^C)\leq \delta\quad\text{when}\;\tau^C=T+\sqrt{\frac{\log(1/\delta)}{2k^+}}.$$%. Then $$\mathds{P}_{S~D}(R_D(\rho^1_S)<T)<\delta.$$    
\end{lemma}

\textit{Proof}. For any $\epsilon\geq 0$, we have 
\begin{align}\label{eq:hoef}
    \mathds{P}_{S\sim D}(R_S(\rho)&-R_D(\rho)\geq\epsilon)=\\\nonumber
    &\mathds{P}_{S^+\sim D^+}(\frac{\sum_i\mathds{I}[X_i\geq\rho]}{k^+}-R_D(\rho)\geq\epsilon)\leq \exp{(-\frac{k^+\epsilon^2}{2})},
\end{align}
Using Hoefding's inequality. 

Now consider the threshold $\bar{\rho}_D=\min\{\rho, R_D(\rho)< T\}$. By Eq.~\ref{eq:hoef}, we have 
\begin{align}\label{eq:hoef_rhobar}
    \mathds{P}_{S\sim D}(R_S(\bar{\rho}_D)-R_D(\bar{\rho}_D)\geq\epsilon)\leq \exp{(-\frac{k^+\epsilon^2}{2})}.
\end{align}
Since $R_D(\bar{\rho}_D)< T$ by definition, we have 
\begin{align}%\label{eq:hoef}
    \mathds{P}_{S\sim D}(R_S(\bar{\rho}_D)\geq T+\epsilon)\leq \exp{(-\frac{k^+\epsilon^2}{2})},
\end{align}
or equivalently, substituting $\delta=\exp{(-\frac{k^+\epsilon^2}{2})},$
\begin{align*}%\label{eq:hoef}
    \mathds{P}_{S\sim D}(R_S(\bar{\rho}_D)\geq T+\sqrt{\frac{\log(1/\delta)}{2k^+}})\leq \delta,
\end{align*}
And therefore,
\begin{align*}%\label{eq:hoef}
    \mathds{P}_{S\sim D}(R_S(\bar{\rho}_D)\geq \tau^C)\leq \delta.\qed
\end{align*}


\textbf{Valid Adjustments using Exact Calculations.} Interestingly, we show that validity can be proven with exact calculations. This follows the observations that $R_S(\bar{\rho}_D)$ is distributed according to a binomial distribution success probability $T$, as discussed below. In the following lemma, $\mathcal{B}(n, p)$ refers to the binomial probability distribution with $n$ samples and probability of success $p$.  

\begin{lemma}
    Let $q(x)=\mathds{P}(\mathcal{B}(k^+, T)\geq x)$ be the tail probability of a binomial distribution with parameters $k^+$ and $T$. Then, $\tau^E=\frac{1}{k^+}\min\{x, q(x)\leq \delta\}$ is a valid adjusted target, i.e., 
    $$\mathds{P}_{S\sim D}(R_S(\rho_D)\geq \tau^E)\leq \delta\quad\text{when}\;\tau^E=\frac{1}{k^+}\min\{x, q(x)\leq \delta\}.$$%. Then 
\end{lemma}

\textit{Proof}. Remember that $R_S(\bar{\rho}_D)=\frac{\sum_i\mathds{I}[X_i\geq\bar{\rho}_D]}{k^+}$. Our main observation is that, even though we don't know the value of $\bar{\rho}_D$, the probability $\mathds{P}(\mathds{I}[X_i\geq\bar{\rho}_D])$ is bounded as 
\begin{align}\label{eq:bound_tail}
    \mathds{P}(\mathds{I}[X_i\geq\bar{\rho}_D])< T.
\end{align}
Eq.~\ref{eq:bound_tail} follows the definition of $\bar{\rho}_D$. Specifically, 
\begin{align*}
    \mathds{P}(\mathds{I}[X_i\geq\bar{\rho}_D])=\sum_{x\in D^+}\frac{\mathds{I}[x\geq\bar{\rho}_D]}{|D^+|}=R_D(\bar{\rho}_D)<T.
\end{align*}
%by definition of $\bar{\rho}_D$, we have that $\frac{\text{\# positive in}\,[\bar{\rho}_D, 1]}{\text{total \# positives}}<T$. Thus, when uniformly sampling over all positive data points, 
Thus, $k^+\times R_S(\bar{\rho}_D)$ is the sum of i.i.d Bernoulli random variables with probability success at most $T$. Consequently, for any $x\geq T$,  $$\mathds{P}_{S\sim D}(R_S(\bar{\rho}_D)\geq x)\leq q(k^+x).$$
Substituting $x=\tau^E$ finishes the proof.\qed

\subsection{Uniform Sampling and Variance-Aware Iterative Selection}
We first generalize the discussion in Sec.XX to present another method to meet the desired recall target. The method, discussed here, follows the general idea of using concentration bounds but it is tighter since it takes into account the variance of observed samples. Since the variance changes at different values of $\rho$, we cannot use a one-off concentration equality to determine an adjusted target, but instead, we need to iteratively calculate confidence intervals for the true mean of the random variable.  

The blue-print for an iterative algorithm is presented in Alg.~\ref{alg:iterative_recall}. Alg.~\ref{alg:iterative_recall} is a generalization of Alg.~\ref{alg:thresh_recall}. It iterates over the data points in ascending order and uses a \textit{discriminator function}, $\lambda$, to decide when to stop. When setting $\lambda(S, \rho)=R_S(\rho)-\tau$ (for either choice of $\tau=\tau^C$ or $\tau=\tau^E$), Alg.~\ref{alg:thresh_recall} becomes equivalent to Alg.~\ref{alg:iterative_recall} (since $R_S(\rho)-\tau$ is monotonically decreasing). However, Alg.~\ref{alg:iterative_recall} allows non-threshold based decision making. Here, we're interested in setting $\lambda(S, \rho)$ to be be function that finds a lower bound $L$ for $\mathds{E}[R_S(\rho)]-T$ with high probability. The algorithm would then find a value of $\rho$ for which $L\geq 0$, which implies  $\mathds{E}[R_S(\rho)]\geq T$.


%Intuitively, Alg.~\ref{alg:thresh_recall} generalizes Alg.~\ref{alg:iterative_recall} in two ways. First, the function $\lambda$ need not depend on $R_S$, allowing us to avoid calculating an unbiased estimator of true recall, which as discussed above, is difficult.  Moreover, it does not require a pre-defined target, $\tau$, but allows decision making based on the observed sample.

We utilize recent advances in calculating confidence intervals for means of bounded random variables, where \cite{waudby2024estimating} shows how to build confidence intervals for the mean of the random variables. The following Lemma is a special case of Theorem 3 by \cite{waudby2024estimating}. 

\begin{lemma}[Theorem 3 by \cite{waudby2024estimating}]%\label{lemma:lb}
    Consider a set of $t$ i.i.d random variables $X=\{X_1, ..., X_t\}$ with $X_i\in[0, 1]$ and $E[X_i]=\mu$ for all $i$. We have% and $\hat{\mu}_u=\max\{m, \mathcal{K}_t(m)<\frac{1}{\delta}\}$
    $$\mathds{P}(\mu<\hat{\mathcal{L}}(X, \delta))\leq \delta \quad\text{for}$$
    %for 
    \begin{align}\label{eq:def_L}
        \hat{\mathcal{L}}(X, \delta)=\min\{m\in[0, 1], \mathcal{K}_i(m)<\frac{1}{\delta}\,\forall i\in[t]\},
    \end{align}
    where, for any $m\in[0, 1]$, 
    \begin{align*}
        \mathcal{K}_t(m)=\Pi_{i=1}^{t}(1+\min(\lambda_i, \frac{3}{4m}))\times(X_i-m), 
    \end{align*}
    \begin{align*}
        %\mathds{P}(\mu\geq W(x))<\delta W(x)=XXXXX\\
        \lambda_i=\sqrt{\frac{2\log(2/\delta)}{k\hat{\sigma}^2_{i-1}}},\; \hat{\sigma}_i^2=\frac{1/4+\sum_{j=1}^i(X_j-\hat{\mu}_j)^2}{i+1}, \;\hat{\mu}_i = \frac{1/2+\sum_{j=1}^iX_j}{i+1}.
    \end{align*}
    %$$\mathds{P}(\mu\notin [\hat{\mu}_l, \hat{\mu}_u]])\leq \delta.$$
    %$$\mathds{P}(\mu\notin\{m, \mathcal{K}_t(m)<\frac{1}{\delta}\})\leq \delta.$$
    %$$\mathds{P}(\mu\geq m\; \text{and}\; \mathcal{K}_t(m)<\frac{1}{\delta})\leq \delta.$$
    %If $$, $\mathds{P}(\mu<M)$
\end{lemma}

We use Lemma~\ref{lemma:lb} to find lower bounds on means of random observations. We note that Theorem 3 by \cite{waudby2024estimating} is more general, and among other generalizations provides a two-sided confidence interval (not just a lower bound on mean as Lemma~\ref{lemma:lb} states). In our analysis, we are only interested in lower bounds and thus have stated a simplification of the result.  

The above lower bound can be used to define $\lambda$ in Alg.~\ref{alg:iterative_recall} to satisfy the desired target recall with the desired probability, as stated below.

%Using Lemma~\ref{lemma:lb} and setting $\lambda(S, \rho)=\hat{\mathcal{L}}(\{\mathds{I}[x\geq\rho], x\in S\})-T$ to XXX, the algorithm  is correct 

\begin{lemma}\label{lemma:unif_iterative}
    Given a desired recall target and probability of failure $\delta$, define
    \begin{align}
        \lambda^U(S, \rho) =\hat{\mathcal{L}}(\{\mathds{I}[x\geq\rho], x\in S\}, \delta)-T.
    \end{align}
    Then, setting $\lambda=\lambda^U$ in Alg.~\ref{alg:iterative_recall}, we have that output of Alg.~\ref{alg:iterative_recall} fails to satisfy recall target $T$ with probability at most $\delta$.
\end{lemma}

\textit{proof}. The algorithm iteratively checks values of $\lambda^U(S, \rho)$ for different $\rho=S[i]$ until  $\lambda^U$ drops to zero. This algorithm returns a set with recall less than $T$ only if $\lambda^U(S, \bar{\rho}_D)\geq 0$, for $\bar{\rho}_D$ defined as Eq.~\ref{eq:rho_d}. Observe that $\lambda^U(S, \bar{\rho}_D)\geq 0$ if and only if $\hat{\mathcal{L}}(\{\mathds{I}[x\geq\bar{\rho}_D], x\in S\}, \delta)\geq T$. By Lemma~\ref{lemma:lb}, we have

$$
\mathds{P}(R_D(\bar{\rho}_D)<\hat{\mathcal{L}}(\{\mathds{I}[x\geq\bar{\rho}_D], x\in S\}, \delta))\leq\delta.
$$
Note that $R_D(\bar{\rho}_D)<T$, so that
$$
\mathds{P}(T<\hat{\mathcal{L}}(\{\mathds{I}[x\geq\bar{\rho}_D], x\in S\}, \delta))\leq\delta,
$$
and consequently 
$$
\mathds{P}(\lambda^U(S, \bar{\rho}_D)\geq 0)\leq\delta,
$$
proving the lemma.\qed

\textbf{Implementation}. Observe that $\mathcal{L}$, as defined in Eq.~\ref{eq:eq:def_L}, requires finding the minimum across potentially infinite values of $m$. In practice in Alg.~\ref{alg:iterative_recall}, we are only using $\mathcal{L}$ to check if $\mathcal{L}(X, \delta)<T$. Consequently, we only need to check if 
\begin{align}\label{eq:check_T}
T\in\{m\in[0, 1], \mathcal{K}_i(m)<\frac{1}{\delta}\,\forall i\in[t]\},
\end{align}
or equivalently if
\begin{align}\label{eq:fast_check}
    \mathcal{K}_i(T)<\frac{1}{\delta}\,\forall i\in[t]
\end{align}
Checking Eq.~\ref{eq:fast_check} is much faster than calculating $\lambda$. 
Note that we can replace Eq.~\ref{eq:check_T} with Eq.~\ref{eq:fast_check} only because the algorithm terminates whenever $\hat{\mathcal{L}}(X, \delta)<T$ so that the algorithm never reaches $\rho$ values for which $T$ is higher than an upper bound for the mean of $R_S(\rho)$. XXX  better phrasing XXXX

\subsection{Proxy Dependent Sampling and Iterative Selection}
In Theorem~\ref{thm:adj_target}, how to adjust the target depends on $k^+$, the number of observed positive samples. The smaller $k^+$ is, the larger the adjusted target will be. This means quality of the result set returned by Theorem~\ref{thm:adj_target} depends on how many positives there are in the dataset. When the total number of positives is small compared with data size, Theorem~\ref{thm:adj_target} may need too many samples to reach a meaningful accuracy. In such a setting, we may want to change our sampling strategy.

Specifically, if the proxy model is well-calibrated, that is, if the scores are correlated with the probability of correctness, then we can hope to sample more positives if the sampling strategy weighs elements based on the proxy scores.

We discuss two solutions to do so. Our first solution uses naive importance sampling, similar to XX, but unlike XXX provides theoretical guarantees. As we discuss below, naive importance sampling can significantly increase variance if there is even small calibration error in the model. This means, an algorithm that provides theoretical guarantees while using naive importance sampling has almost no utility. To address this issue, we propose clamped importance sampling, tha combined clamping with importance sampling to reduce the variance. This approach increases bias but reduces variance, where we quantify the bias in terms of model calibration error. This approach provides theoretical guarantees that depend on the model calibration error.



\subsubsection{Importance Sampling}
Importance sampling operates as follows. Consider a function $f$, and assume we are interested in $\mathds{E}_{x\sim u}[f(x)]$. Instead of sampling the data according to $u$, we can sample the data using another data distribution with p.m.f $w$. We have $\mathds{E}_{x\sim u}[f(x)]=\mathds{E}_{x\sim w}[f(x)\frac{u(x)}{w(x)}]$.  In other words, we can estimate $\mathds{E}_{x\sim u}[f(x)]$ by sampling the data from a new distribution $w$ and reweight our estimates to get an unbiased estimator of the data from the original distribution $u$. 

However, there are many challenges in analyzing importance sampling. Consider the approach in Sec.XXX, where we consider sampling only positives from the data. In that case, $u(x)$ is the uniform distribution over the positives, and $w(x)$ is another distribution also over the positives. This means, both $u(x)$ and $w(x)$ will be unknown, given that we do not know apriori which points are positives, so that we cannot even compute $f(x)\frac{u(x)}{w(x)}$. On the other hand, one can consider the ratio of two random variables view of recall. However, in such a setting $\mathds{E}_{x\sim u}[R_S(\rho)]\neq R_D(\rho)$ since $\mathds{E}_{x\sim u}[R_S(\rho)]$ is the expected value of ratio of two random variables and not necessarily equal to the ratio of their respective expected values. 

The above challenges make it difficult to apply the same techniques as before when performing importance sampling. Nonetheless, we show that a careful selection of $\lambda$ in our iterative selection algorithm does the trick. Let $\zeta=\sum_{x\in D^+}\mathcal{P}(x)$.

Add analogs to before, discuss unboundedness, also the fact that this is over positives

\begin{lemma}%\label{lemma:importance_sampling}
    Define $\mathbf{Z}^\rho=\{\bar{Z}_1^\rho, ..., \bar{Z}_{k^+}^\rho\}$ where
    $$
    \bar{Z}_i^\rho =\psi Z_i+T,\; \text{where}\;\; Z_i^\rho = \frac{\mathds{I}[X_i>\rho]-T}{\mathcal{P}(X_i)},
    $$
    $$
    \text{with}\; \psi\; \text{as either}\; \psi=\min_{x\in D}\mathcal{P}(x)\; \text{or}\; \psi=\min_{x\in D^+}\mathcal{P}(x).
    $$
    Let $$\lambda^I(S, \rho)=\hat{\mathcal{L}}(\mathbf{Z}^\rho, \delta)-T.$$ 
    Then, Alg.~\ref{alg:iterative_recall}, sampling data according to $\mathcal{W}(x)=\frac{\mathcal{P}(x)}{\zeta}$ and with $\lambda=\lambda^I$ returns a set of elements with recall less than $T$ with probability at most $\delta$.
\end{lemma}

\textit{Proof.} The proof follows a similar argument as Lemma~\ref{lemma:unif_iterative}. The Alg~\ref{alg:iterative_recall} fails to achieve the recall target only if $\lambda^I(S, \bar{\rho}_D)\geq 0$, or equivalently $\hat{\mathcal{L}}(\mathbf{Z}^{\bar{\rho}_D}, \delta)\geq T$. We show that this happens with probability at most $\delta$. To show this, assume for now that 
\begin{align}\label{eq:expected}
\mathds{E}[\bar{Z}_i^{\bar{\rho}_D}]<T.
\end{align} 
Combining this with Lemma~\ref{lemma:lb} proves that $\mathds{P}(\hat{\mathcal{L}}(\mathbf{Z}^{\bar{\rho}_D}, \delta)\geq T)\leq \delta.$ Note that $\bar{Z}_i^\rho$ is a normalization of $Z_i^\rho$ to fall between 0 and 1 so that Lemma~\ref{lemma:lb} can be applied.

It remains to show Eq.~\ref{eq:expected}. Consider any $\rho$, and note that $\psi$ and $T$ are constants, so we only need to focus on $Z_i^{\rho}$. We have
\begin{align*}
    \mathds{E}[Z_i^{\rho}]=&\mathds{E}_{X_i\sim \mathcal{W}}[\frac{\mathds{I}[X_i>\rho]-T}{\mathcal{P}(X_i)}]\\
    =&\mathds{E}_{X_i\sim \mathcal{W}}[\frac{\mathds{I}[X_i>\rho]}{\mathcal{P}(X_i)}]-\mathds{E}_{X_i\sim \mathcal{W}}[\frac{T}{\mathcal{P}(X_i)}]
\end{align*}
First, consider the first term
\begin{align*}
    \mathds{E}_{X_i\sim \mathcal{W}}[\frac{\mathds{I}[X_i>\rho]}{\mathcal{P}(X_i)}]&=\sum_{p\in D^+}\frac{\mathds{I}[p>\rho]}{\mathcal{P}(p)}\frac{\mathcal{P}(p)}{\zeta}\\&=\frac{|D^+|}{\zeta}R_D(\rho).
\end{align*}
For the second term
\begin{align*}
    \mathds{E}_{X_i\sim \mathcal{W}}[\frac{T}{\mathcal{P}(X_i)}]&=T\sum_{p\in D^+}\frac{1}{\mathcal{P}(p)}\frac{\mathcal{P}(p)}{\zeta}=\frac{|D^+|}{\zeta}T.
\end{align*}
So that
\begin{align}\label{eq:z_expected}
    \mathds{E}[Z_i^\rho]=\frac{|D^+|}{\zeta}(T-R_D(\rho))
\end{align}
Substituting back, we have 
$$
\mathds{E}[\bar{Z}_i^{\bar{\rho}_D}]=\psi\frac{|D^+|}{\zeta}(R_D(\bar{\rho}_D)-T)+T.
$$
Note that $R_D(\bar{\rho}_D)<T$  by definition, so
$$
\psi\frac{|D^+|}{\zeta}(R_D(\bar{\rho}_D)-T)<0
$$
and therefore $\mathds{E}[\bar{Z}_i^{\bar{\rho}_D}]<T$ as desired.\qed




\textbf{Challenges with Importance Sampling.} Observe that in Lemma~\ref{lemma:importance_sampling} our random variables depend on inverse of $\mathcal{P}$. This means, if the proxy score for a positive sample is lower, the value of the random variable can significantly explode, leading to high variance in the estimator. The following Lemma quantifies the variance. 
\begin{lemma}%\label{lemma:importance_variance} 
Consider the random variable $Z_i^\rho$ from Lemma~\ref{lemma:importance_sampling} for any $\rho\in[0, 1]$. We have
\begin{align*}
    \frac{\kappa}{\zeta}+\frac{T^2}{\zeta}\sum_{x<\rho}\frac{1}{\mathcal{P}(x)}\leq Var(Z_i^\rho)\leq \frac{\kappa}{\rho\zeta}+\frac{T^2}{\zeta}\sum_{x<\rho}\frac{1}{\mathcal{P}(x)},
\end{align*}
for $\kappa=|D^+|((1-T)^2R_D(\rho)+T-R_D(\rho))$.
\end{lemma}

\textit{Proof.} We have
\begin{align*}
    Var(Z_i^\rho)=\mathds{E}[(Z_i^\rho)^2)]-\mathds{E}[Z_i^\rho]^2
\end{align*}
The expected value in the second term is calculated in Eq.~\ref{eq:z_expected}, so consider the first term. We have
\begin{align*}
    \mathds{E}[(Z_i^\rho)^2)]&=\mathds{E}_{X_i\sim \mathcal{W}}[(\frac{\mathds{I}[X_i>\rho]-T}{\mathcal{P}(X_i)})^2]\\
    &=\sum_{x\in D^+}(\frac{\mathds{I}[X_i>\rho]-T}{\mathcal{P}(X_i)})^2\frac{\mathcal{P}(x)}{\zeta}=\frac{1}{\zeta}\sum_{x\in D^+}(\frac{\mathds{I}[X_i>\rho]-T)^2}{\mathcal{P}(X_i)})\\
    &=\frac{(1-T)^2}{\zeta}\sum_{x\geq\rho}\frac{1}{\mathcal{P}(x)}+\frac{T^2}{\zeta}\sum_{x<\rho}\frac{1}{\mathcal{P}(x)}.
\end{align*}
Now observe that 
$$
R_D(\rho)|D^+|\leq\sum_{x\geq\rho}\frac{1}{\mathcal{P}(x)}\leq \frac{R_D(\rho)|D^+|}{\rho}.
$$
This, together with Eq.~\ref{eq:z_expected}, yields the result.\qed

Importantly, observe the dependence on $\frac{1}{\mathcal{P}(x)}$ in Lemma~\ref{lemma:importance_variance} for $x<\rho$. Recall that our analysis in Lemma~\ref{lemma:importance_sampling} depended on $Z_i^{\bar{\rho}_D}$. Using $\bar{\rho}_D$ in Lemma~\ref{lemma:importance_variance}, implies that the approach is particularly sensitive to proxy scores smaller than $\bar{\rho}_D$ for positive records. By definition of $\bar{\rho}_D$, more than $1-T$ percent of the positives are have scores smaller than $\bar{\rho}_D$. Even if one such a positive record has $\mathcal{P}(x)$ close to zero, $Var(Z_i^{\bar{\rho}_D})$ becomes extremely large, leading to an estimator with little utility. Since, in practice, models are uncalibrated and $\mathcal{P}(x)$ can be small for positive samples, using the importance sampling approach, s discussed above often performs poorly.

\subsubsection{Lower bound}
\begin{lemma}\label{lemma:recall_rho_must_be_zero_general}
Consider any algorithm $A$ that samples a set of, $k$, points $S$, and returns a cascade threshold $\rho_{S, D}$ based on the observed labels, $\{\mathcal{O}(x);x\in S\}$, and all proxy scores $\{\mathcal{S}(x);x\in D\}$. If $\mathds{P}_{S\sim D}(\mathfrak{R}_D(\rho_{S, D})\leq T)\leq \delta$ for all possible datasets of size $N$ and with $N^+$ positives, then we must have $\mathds{P}_{S\sim D}(\mathfrak{P}_D(\rho_{S, D})\geq \frac{N^+}{N-t})\leq \alpha_t-\delta$ for any $t\geq\frac{N^+}{2})$ with $\frac{N^+}{2}$-th lowest proxy score and $\alpha_t$ denotes the probability that the algorithm does not sample any point with proxy score in $[0, x_t]$. Specifically, if sampling $k$ points i.i.d, where each point is sampled with probability $W(x)$ where $\mathcal{W}$ is increasing in $\mathcal{S}(x)$, we have $\alpha\leq(1-\frac{(1-T)t}{N})^k$.
\end{lemma}

\textit{Proof.} Let $D^i\subseteq i$, $i\in[n]$ be the subset of $D$ consisting of points with proxy scores at most equal to the $i$-th lowest proxy of points in $D$. First, consider the case that $\sum_{x\in D^t}\mathds{I}[\mathcal{O}(x)=1]\geq N^+\times(1-T)$. To obtain recall at least $T$, we must have $\rho_{S, D}\in [0, x_t]$ so that $\mathds{P}(\rho_{S, D}\in [0, x_t])\geq 1-\delta$. Note that precision where $\rho_{S, D}\in[0, x_t]$ is at most $\frac{N^+}{N-t+(1-T)N^+}$, so that $\mathds{P}(\mathfrak{P}_D(\rho_{S, D})\leq \frac{N^+}{N-t+(1-T)N^+})\geq 1-\delta$, proving the result for this case. 

Next consider the case where $\sum_{x\in D^t}\mathds{I}[\mathcal{O}(x)=1]< N^+\times(1-T)$.
%Now consider a dataset $D$ where less than $\frac{N^+}{2}$ number of positive samples are in the range $[0, t]$. 
Assume for the purpose of contradiction that $\mathds{P}(\rho_{S, D}\in [0, x_t])< \alpha-\delta$, that is the algorithm returns a threshold in $[0, x_t]$ wit probability less than $\alpha-\delta$. This means that $$\mathds{P}(S\cap D^t=\emptyset,\; \rho_{S, D}\in [0, x_t])< \alpha-\delta,$$
where $S\cap D^i=\emptyset$ is the event that the algorithm does not sample any point with proxy score in $[0, x_t]$.% and returns a threshold in $[0, t]$ is also bounded by $\alpha-\delta$. 
Using the above Eq.~\ref{eq:no_sample_but_more_than_t}, we construct a dataset, $\bar{D}$, on which the algorithm fails with probability more than $\delta$. Consider the dataset $\bar{D}$ with the same proxy score and labels as $D$, except that all points with proxy scores in $[0, x_t]$ have a positive label. Note that the total number of positives in $\bar{D}$ is at most $N^++t$ with at least $t$ of the positives in $[0, x_t]$. Thus, a cascade threshold $\rho_{S, D}>x_t$ leads to a recall at most $\frac{N^+}{N^++t}=\frac{1}{1+\frac{t}{N^+}}\leq \frac{1}{2-T}$, because $t\geq N^+\times(1-T)$. Note that  $\frac{1}{2-T}<T$ for $T\geq 0.5$. Therefore,
\begin{equation}\label{eq:error_if_more_than_t}
\mathds{P}(\mathfrak{R}_D(\rho)<T)\geq\mathds{P}(\rho_{S, \bar{D}}\in (x_t, 1])
\end{equation}


Since $\rho_{S, D}$ is chosen deterministically given the observed samples, $\rho_{S, D}$ is identically selected for datasets with the same proxy score and the same observed labels. $D$ and $\bar{D}$ are identical except for labels in $[0, x_t]$ so whenever running the algorithm on $\bar{D}$ but for any $S$ where $S\cap\bar{D^t}=\emptyset$, we must have $\rho_{S, \bar{D}}=\rho_{S, D}$. Thus consider
\begin{align*}
    \mathds{P}(\rho_{S, \bar{D}}\in (x_t, 1])&\geq \mathds{P}(S\cap\bar{D}^t=\emptyset,\;\rho_{S, \bar{D}}\in (x_t, 1])\\
    &=\mathds{P}(S\cap\bar{D}^t=\emptyset)-\mathds{P}(S\cap\bar{D}^t=\emptyset,\;\rho_{S, \bar{D}}\in [0, x_t])\\
    &=\mathds{P}(S\cap D^t=\emptyset)-\mathds{P}(S\cap D^t=\emptyset,\;\rho_{S, D}\in [0, x_t])\\
    &>\alpha-(\alpha-\delta)=\delta.
\end{align*}
Thus, combining the above with Eq.~\ref{eq:error_if_more_than_t}, we see that the algorithm fails with probability more than $\delta$ on $\bar{D}$, causing a contradiction. Thus, we must have $\mathds{P}(\rho_{S, D}\in [0, x_t])\geq \alpha-\delta$, which as discussed before, implies $\mathds{P}(\mathfrak{P}_D(\rho_{S, D})\leq \frac{N^+}{N-t+(1-T)N^+})\geq \alpha-\delta$.

Finally, note that if samples are selected i.i.d, with the probability increasing in proxy scores, then the probability that any sample is one of the first $t$ data points is at most $\frac{t}{N}$, so that, $\alpha$, the probability of not selecting any of the first $t$ data points in $k$ samples is at least $\alpha\geq (1-\frac{t}{N})^k$. \qed

\subsubsection{Clamped Importance Sampling}
A natural solution to the problem with importance sampling is to avoid sampling from records with low proxy scores. The accuracy of such a solution depends on how well-calibrated the proxy model is. 

We first describe an approach that provides gaurantees based on assumptions on model caliberation. We then discuss how such model caliberation assumptions can be validated using sampling.

\textbf{Calibration Dependent Sampling}. First, we define a measure of calibration that is intuitive and useful for our setting. XXX CHECK MAYBE THERE IS SOMETHIING LIKE THIS

\begin{definition}
    Consider $\alpha\in [0, n]$ and the subset $\{x_1, ..., x_{i_\alpha}\}$ of $D$ where $i$ is the largest integer such that $\sum_{j=1}^i\mathcal{P}(x)\leq \alpha.$. We say that the proxy model $\mathcal{P}$ is $(\alpha, \beta)$-calibrated with respect to dataset $D$ if for the subset $\sum_{j=1}^{i_\alpha}\mathcal{O}(x_i)\leq \beta+\alpha$.
\end{definition}

Intuitively, if proxy scores are taken as probability that a sample is positive, then $(\alpha, \beta)$-calibration means, for a subset of $D$ whose expected number of positive samples is $\alpha$, the actual number of positive samples are at most $\alpha+\beta$. In practice, this notion allows us to bound the number of positive samples with low scores so that we can only perform sampling on elements with high enough proxy scores. The following Lemma states this formally.

\begin{lemma}\label{lemma:clamped}
    Assume the proxy model is $(\alpha, \beta)$-calibrated and that there are at least $\gamma$ number of true positives. Then, sampling data records with proxy score $[\alpha, 1]$ and using the target $T'=T(1+\frac{\alpha+\beta}{\gamma-(\alpha+\beta)})$ yields an algorithm that meets the target $T$ with probability $\delta$. 
\end{lemma}

\textit{Proof}. By assumption, there are at most $\alpha+\beta$ positive records in $[0, \alpha]$, and there are at least $\gamma-(\alpha+\beta)$ positives in $[\alpha, 1]$. Assume the algorithm guarantees recall $T'$ for records in $[\alpha, 1]$. Let $c$ be the total number of positives in $[\alpha, 1]$ and $c_R$ be the true positives returned by the algorithm. We have, $T'\leq\frac{c_R}{c},$ and note that $c\geq \gamma-(\alpha+\beta)$.

By definition of $T'$, 
\begin{align*}
    \frac{c_r}{c}\geq T'=T(1+\frac{\alpha+\beta}{\gamma-(\alpha+\beta)})\geq T(1+\frac{\alpha+\beta}{c}).
\end{align*}
Consequently, for the recall over the entire set $\frac{c_R}{c+(\alpha+\beta)}\geq T$ as desired. \qed

XXXXXX In practive, we show that common models are often $\alpha, \beta$ calibrated for large values of $\alpha$ and small values of $\beta$. We set $\alpha=1$ and $\beta=0$. This is better than setting threshold upper bound because that way there's no room for error. This is less restrictive and also doesn't depend on actual values so we can set this data independently.  

\textbf{Estimating Calibration}. Finally, to avoid assumptions on model calibration an number of ground-truth samples, one can estimate $\beta$ by sampling. This requires dividing the sampling budget into two, $k_1$ and $k_2$ and also choosing an $\alpha$ values. Then, we can use the $k_1$ samples to estimate the total number of positives in $x_1$, .., $x_{i_\alpha}$. Then, we can use $k_2$ samples to estimate a recall threshold. The algorihtm remains the same, but this simply changes the $\beta$ value used in Lemma~\ref{lemma:clamped}. We need to use union bound to gaurantee correctness so $\delta$ has to be divided by two in each case.

Finally, $\gamma$ can also be estimated from observations. In practice, one can simply use to the total number of observed positives as $\gamma$. Given that a small $\gamma$ is typically good enough (e.g., $\gamma~100$ in our experiments), estimating the true number of ground-truth obervtion is not necessary. 

May need to do btter on how to aloocate budge 


XXX Better, will likely need an algorithm somewhere. Need to also add to experiment.s 

XXXX at least experimentally figure out if importance sampling is useful, how does it change variance as psi goes down, either with knowledge of minimum of positive or without knowledge of minimum of positive

\if 0
\begin{theorem}
    Consider a uniform sample $S\sim D$, and let $p$ be the number of positives in $S$, i.e., $p=|\{x\in S, O(x)=1\}|$. Set $$\tau^*=\max \{\tau\in[0, 1], \text{where}\, \mathds{P}(\mathds{B}(p, T)\geq p\tau)\leq \delta\},$$ and find $$\rho^*=\max\{\rho\in[0, 1] where R_S(\rho)\geq\tau^*\}$$
\end{theorem}
\fi
